# Supplementary material for: Inclusive Deep Inelastic Scattering at High Q2 with Longitudinally Polarised Lepton Beams at HERA
Source: arXiv:1206.7007 source file (2012-06-29)
Supplement: Supplementary file 1 [file Appendix.tex]

%---------------------------------------
\appendix
\section{Treatment of H1 Correlated Systematic Uncertainties in QCD Analysis}
\label{sec:append}

The correlated systematic uncertainties for the H1 cross section
measurements may be correlated across data sets since they may arise
from the same source and are not treated independently in the QCD
analysis presented here. The relationship between the error sources as
used in the fitting procedure is summarised in table~\ref{tab:qcdsys} for
each of the seven correlated systematics considered. This leads to $18$
independent error sources. Note that all H1 quoted luminosity
uncertainties have a common contribution of $0.5\%$ arising from the
theoretical uncertainty of the Bethe-Heitler cross section. This common
contribution has been taken into account in the QCD analysis.

\begin{table}[htp]
\begin{center}
\begin{tabular}{|ll|cccccccc|}
\hline
 data set & reaction & $\delta \mathcal{L}$ &   $\delta^E$ & $\delta^{\theta}$ &  $\delta^h$
 &$\delta^N$&
$\delta^B$& $\delta^V$& $\delta^S$ \\ \hline
min bias     $97$  &  $e^+p$ NC & $\mathcal{L}1$ & $E1$ &$\theta1$ & $h1$ & $N1$ & $B1$ & $--$ & $--$ \\
low $Q^2$  $96-97$ &  $e^+p$ NC & $\mathcal{L}2$ & $E1$ &$\theta1$ & $h1$ & $N1$ & $B1$ & $--$ & $--$ \\
high $Q^2$ $94-97$ &  $e^+p$ NC & $\mathcal{L}3$ & $E2$ &$\theta2$ & $h2$ & $N1$ & $B2$ & $--$ & $--$ \\
high $Q^2$ $94-97$ &  $e^+p$ CC & $\mathcal{L}3$ & --   &   --     & $h2$ & $N1$ & $B2$ & $V1$ & $--$ \\
high $Q^2$ $98-99$ &  $e^-p$ NC & $\mathcal{L}4$ & $E2$ &$\theta3$ & $h2$ & $N1$ & $B2$ & $--$ & $S1$ \\
high $Q^2$ $98-99$ &  $e^-p$ CC & $\mathcal{L}4$ & --   &   --     & $h2$ & $N1$ & $B2$ & $V2$ & $--$ \\
high $Q^2$ $99-00$ &  $e^+p$ NC & $\mathcal{L}5$ & $E2$ &$\theta3$ & $h2$ & $N1$ & $B2$ & $--$ & $S1$ \\
high $Q^2$ $99-00$ &  $e^+p$ CC & $\mathcal{L}5$ & --   &   --     & $h2$ & $N1$ & $B2$ & $V2$ & $--$ \\
\hline                                                       
\end{tabular}        
\end{center}
\caption 
 {\label{tab:qcdsys} \sl For each correlated systematic error source listed, the
    correlation across H1 data sets is shown. For each of the eight
    correlated systematic error sources one or more parameters is
    included in the QCD fit procedure. The sources considered are due to
    the luminosity uncertainty ($\delta^{\mathcal{L}}$) electron energy
    uncertainty ($\delta^E$), the electron polar
    angle measurement ($\delta^{\theta}$), the hadronic energy
   uncertainty ($\delta^{h}$), the uncertainty due to noise subtraction
   ($\delta^{N}$), the background subtraction error ($\delta^{B}$), the
    uncertainty in measurement of the ratio $V_a/V_{ap}$ ($\delta^{V}$),
    and the error of the background subtraction charge asymmetry
    ($\delta^{S}$). The table entries indicate the correlation of the
    error sources across the H1 data sets. For example, the uncertainty
    due to the noise subtraction is the same for all data sets leading
    to one common parameter in the fit ($N1$), whereas the electron
    energy uncertainty has two independently varying parameters ($E1$
    and $E2$) for the H1 NC data sets only.}
\end{table}

% \begin{table}[h]
% \footnotesize
% \begin{tabular}{ll}
% & \underline{sources of systematic uncertainties:}\\[.5mm]
% $E_{el}$: &  electron energy calibration \\[-.5mm]
% $\theta_{el}$: &  polar angle of electron measurement\\[-.5mm]
% $E_{had}$ : &  hadronic energy calibration \\[-.5mm]
% Noise: &  noise suppression algorithm\\[-.5mm]
% BG: &  background estimate by Monte Carlo\\[-.5mm]
% Vap: &  anti $\gamma p$ cut \\[-.5mm]
% Asy: &  background elimination by subtraction of\\[-.5mm]
%      & the wrong charge lepton candidates\\[-.5mm]
% \end{tabular}
% \end{table}
